# Supplementary material for: Optimizing Ordered Graph Algorithms with GraphIt
Source: arXiv:1911.07260 source file (2020-01-26)
Supplement: Supplementary file 1 [file appendix.tex]

\section{Appendix}
\label{sec:appendix}

\begin{figure*}[t]
\centering
%\hspace{2em}
    \includegraphics [width=0.7\textwidth] {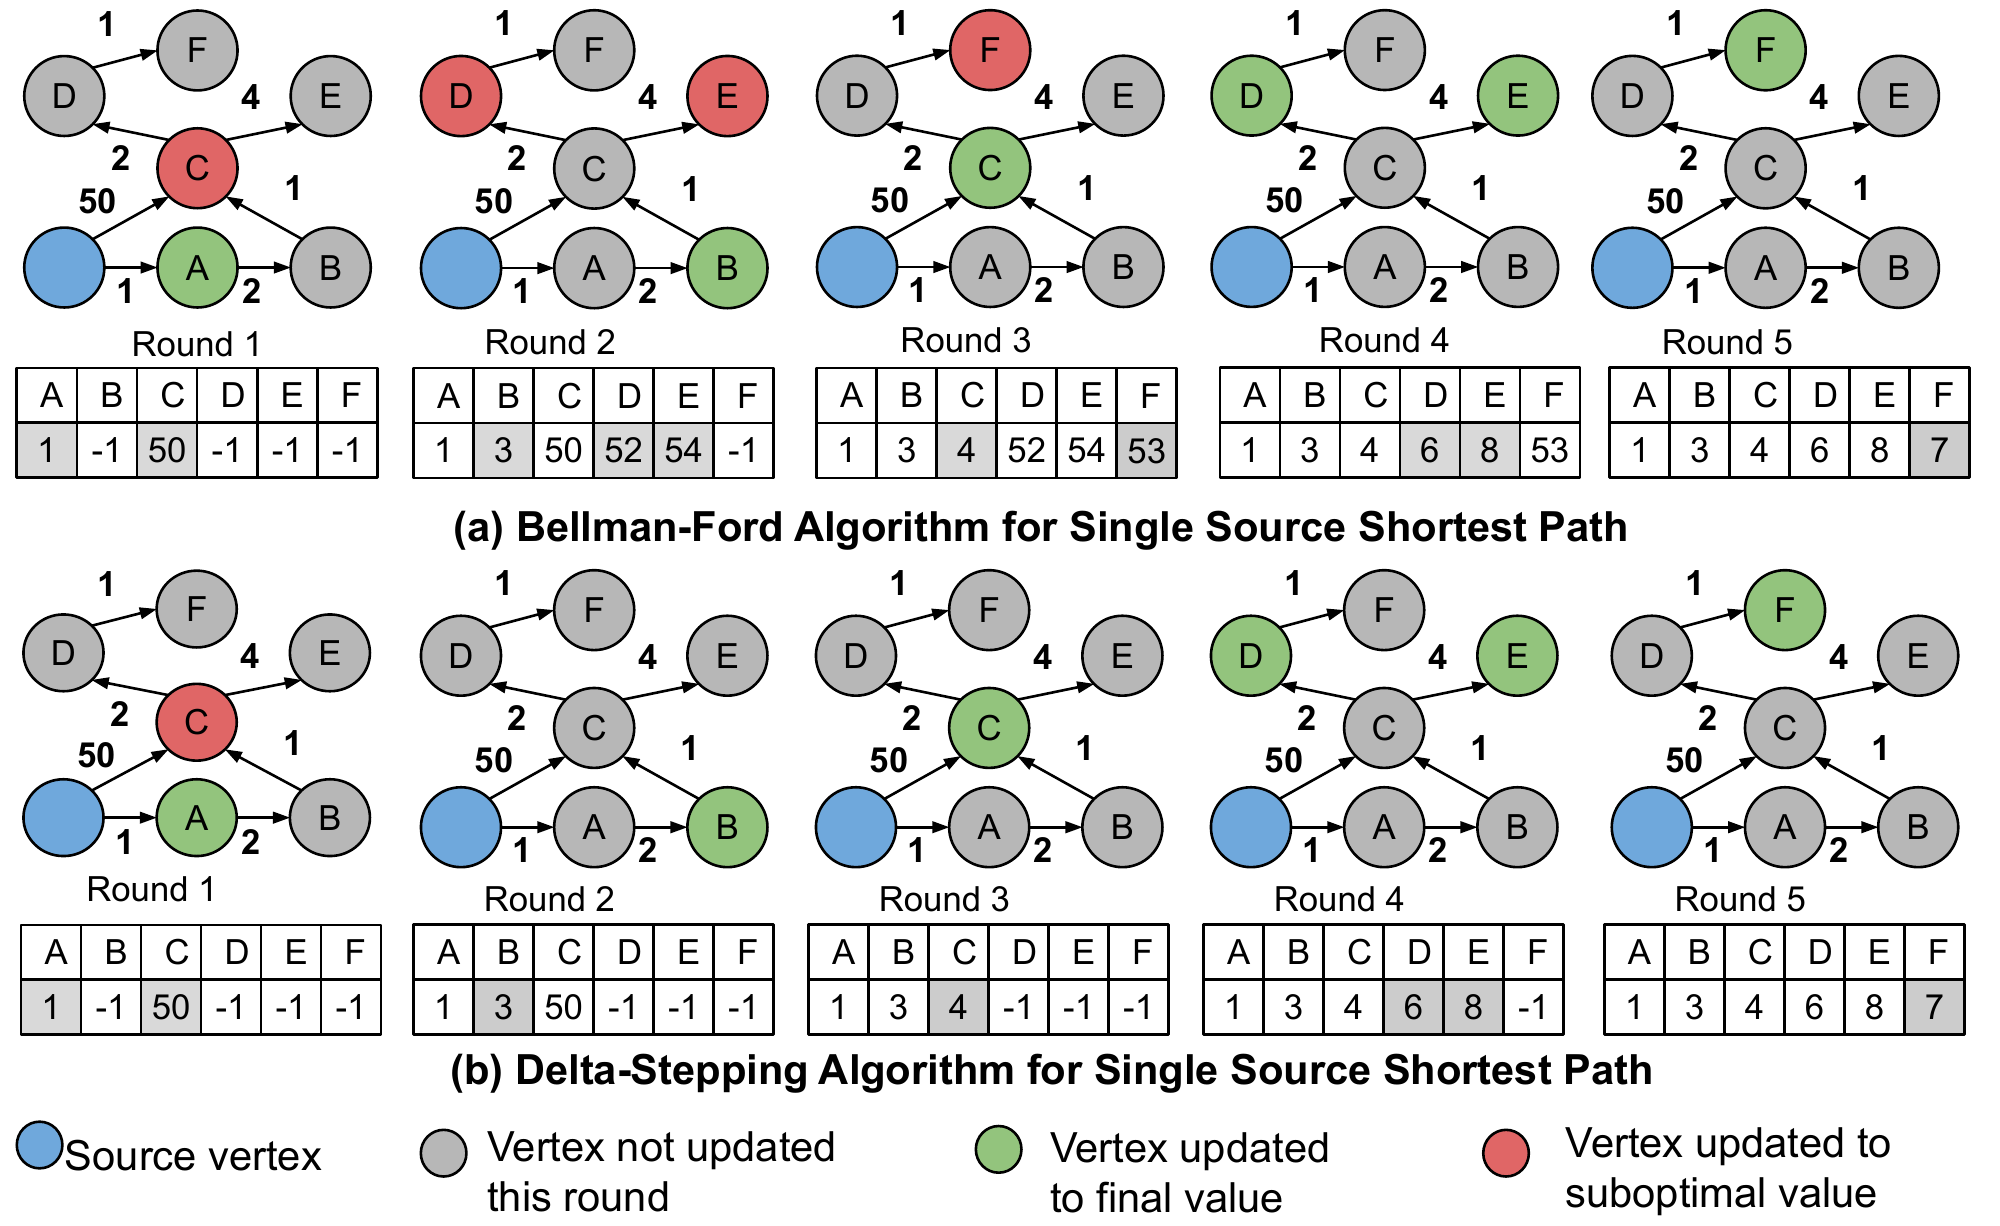}
    \caption{SSSP implemented with Bellman-Ford and \deltastepping{} ($\Delta = 30$). The distances are shown in the tables. Bellman-Ford needs 10 updates, whereas \deltastepping{} needs only 7 updates.}
    \label{fig:delta_stepping_demo}
\end{figure*}

\subsection{Bellman-Ford vs \deltastepping{}}

We use Figure~\ref{fig:delta_stepping_demo} to demonstrate the difference between Bellman-Ford (unordered algorithm) and \deltastepping{} (ordered algorithm) for SSSP. 
Bellman-Ford updates the distance to vertex $C$ in round 1, and then immediately propagates updates to vertices $D$, $E$, and $F$ in both rounds 2 and 3.
However, these updates (highlighted in red) constitute wasted work.
, since vertex $C$'s correct shortest path distance is set through a 3-hop path through vertices $A$ and $B$.
\deltastepping{} only propagate updates to vertices $D$, $E$, and $F$ after the distance to vertex $C$ is finalized in round 3.
\deltastepping{} sacrifices some parallelism, but avoids redundant updates, leading to significant speedup over Bellman-Ford on many graphs.
\deltastepping{} can often achieve significant speedup over Bellman-Ford on many graphs.

\subsection{Schedules and Parameters used in Evaluation}

% priority coarsening factor for different graphs and different frameworks 

% single socket vs two socket performances
\myparagraph{SSSP, PPSP, wBFS, \astar{}} For SSSP, PPSP, \astar{} in Julienne and GAPBS, we used the single socket performance on the road networks (MA, GE, RD), and the two-socket performance on the social networks and web graphs. 
Using both sockets results in more than 4$\times$ slowdown for these two frameworks on the road networks. 
We used the \texttt{no\_dense} flag for Julienne on wBFS and SSSP for the best performance. 
\OG and Galois's performances scale across two sockets for all graphs. 
We used eager bucketing with bucket fusion for SSSP, PPSP, wBFS, and \astar{}  for \OG on all graphs except for the smaller social networks (Live Journal and Orkut), and we used a merge threshold of 1000.

% number of buckets used 
\myparagraph{\kcore and SetCover} Both \OG and Julienne adopt the lazy bucketing strategy for \kcore and SetCover. 
For \kcore, we used 16 open buckets for both \OG and Julienne for all graphs. 
We found that using 16 buckets outperform using 128 of buckets by 10-20$\%$. 
For SetCover, we used 128 buckets, which outperform 16 buckets by up to 2$\times$.

\begin{figure}[t]
\begin{lstlisting} [language=graphit,escapechar=|]
element Vertex end
element Edge end
const edges : edgeset{Edge}(Vertex, Vertex) = load(argv[1]);
const vertices : vertexset{Vertex} = edges.getVertices();
const D: vector{Vertex}(uint) = edges.getOutDegreesUint();
const pq: priority_queue{Vertex}(uint);
func apply_f(src: Vertex, dst: Vertex)
    var k: int = pq.get_current_priority();
    pq.updatePrioritySum(dst, -1, k);
end
 
func main()
	pq = new priority_queue{Vertex}
	    (uint)(false, "lower_first", D);
	var finished: int = 0; 
	while (finished != vertices.size()) 
        var frontier: vertexset{Vertex}= pq.dequeue_ready_set();
        finished += frontier.getVertexSetSize();
        #s1# edges.from(frontier).applyUpdatePriority(apply_f);
        delete frontier;
	 end
end
\end{lstlisting}
\caption{\OG algorithm for \kcore{}. }
\label{fig:code:kcore_GraphIt}
\end{figure}

\begin{figure}[t]
\begin{lstlisting} [language=graphit,escapechar=|]
element Vertex end
element Edge end
extern func load_coords(filename: string, num_nodes: int);
extern func calc_dist(src: Vertex, dst: Vertex) -> output: double;
const edges : edgeset{Edge}(Vertex,Vertex, int) = load(argv[1]);
const vertices : vertexset{Vertex} = edges.getVertices();
const f_score : vector{Vertex}(int) = INT_MAX; 
const g_score : vector{Vertex}(int) = INT_MAX; 
const dst_vertex : Vertex;
const pq: priority_queue{Vertex}(int);

func updateEdge(src : Vertex, dst : Vertex, weight : int)
    var new_f_score : int = f_score[src] + weight;
    var changed : bool = writeMin(f_score, dst, new_f_score);
    if changed
        var new_g_score : int = max(new_f_score + 
            calc_dist(dst, dst_vertex), g_score[src]);
        pq.updatePriorityMin(dst, g_score[dst], new_g_score);
    end
end

func main()
    var start_vertex : int = atoi(argv[2]);
    dst_vertex = atoi(argv[3]);
    load_coords(argv[1], edges.getVertices());
    f_score[start_vertex] = 0;
    g_score[start_vertex] = calc_dist(start_vertex, dst_vertex);
    pq = new priority_queue{Vertex}(int)
        (true, "lower_first", g_score, start_vertex);
    while (pq.finishedNode(dst_vertex) == false)
        var frontier : vertexset{Vertex} = pq.dequeue_ready_set();
        #s1# edges.from(frontier).applyUpdatePriority(updateEdge);
        delete frontier;
    end
end
\end{lstlisting}
\caption{\OG algorithm for \astar{}. }
\label{fig:code:astar_GraphIt}
\end{figure}

\subsection{Additional Algorithms in \OG}
Figure~\ref{fig:code:kcore_GraphIt} and Figure~\ref{fig:code:astar_GraphIt} show the \OG implementation of 
ordered \kcore{} and \astar{} algorithms. 
\kcore{} computes all the cores in the graph. 
\astar{} computes the shortest distance between a start and end point.
\astar{} uses an extern function defined in C++, \texttt{calc\_dist}, to compute the estimated 
distance from the current point to the destination point.
